# Supplementary material for: Pick-and-Mix Information Operators for Probabilistic ODE Solvers
Source: arXiv:2110.10770 source file (2021-10-20)
Supplement: Supplementary file 1 [file supplementary.tex]

% Created 2021-05-15 Sa 20:07
% Intended LaTeX compiler: pdflatex
\documentclass[twoside]{article}
\usepackage{aistats2022}

\usepackage[round]{natbib}

\bibliographystyle{apalike}

\input{preamble.tex}

% xr-hyper:
\externaldocument{paper}

\begin{document}

\input{supplement_content}

\bibliography{references}

\end{document}
